# Supplementary material for: Using protein blocks to build custom fragment libraries from protein structures
Source: arXiv:2005.01696 source file (2025-07-19)

## Supplementary Figures 1. Coverage density plots.

The plots under this heading show the distribution of the number of fragments per position. The analysis has been performed for both treatment of the query proteins: (1) Protein Block Assignment (PBA) and (2) Protein Block Prediction (PBP). The graphs are further classified into section : (a) SCOP Class – all  $\alpha$ , (b) SCOP Class – all  $\beta$ , (c) SCOP Class -  $\alpha + \beta$  and (d) SCOP Class -  $\alpha/\beta$ . The percentage of coverage for each test protein is marked above the plot. Along with it the positions for each protein with no fragment hits are marked in red and the number of residues with no hits is also shown above each graph.

### Supplementary Figure 1.1a

Protein Block Assignment (PBA) - SCOP Class – all  $\alpha$

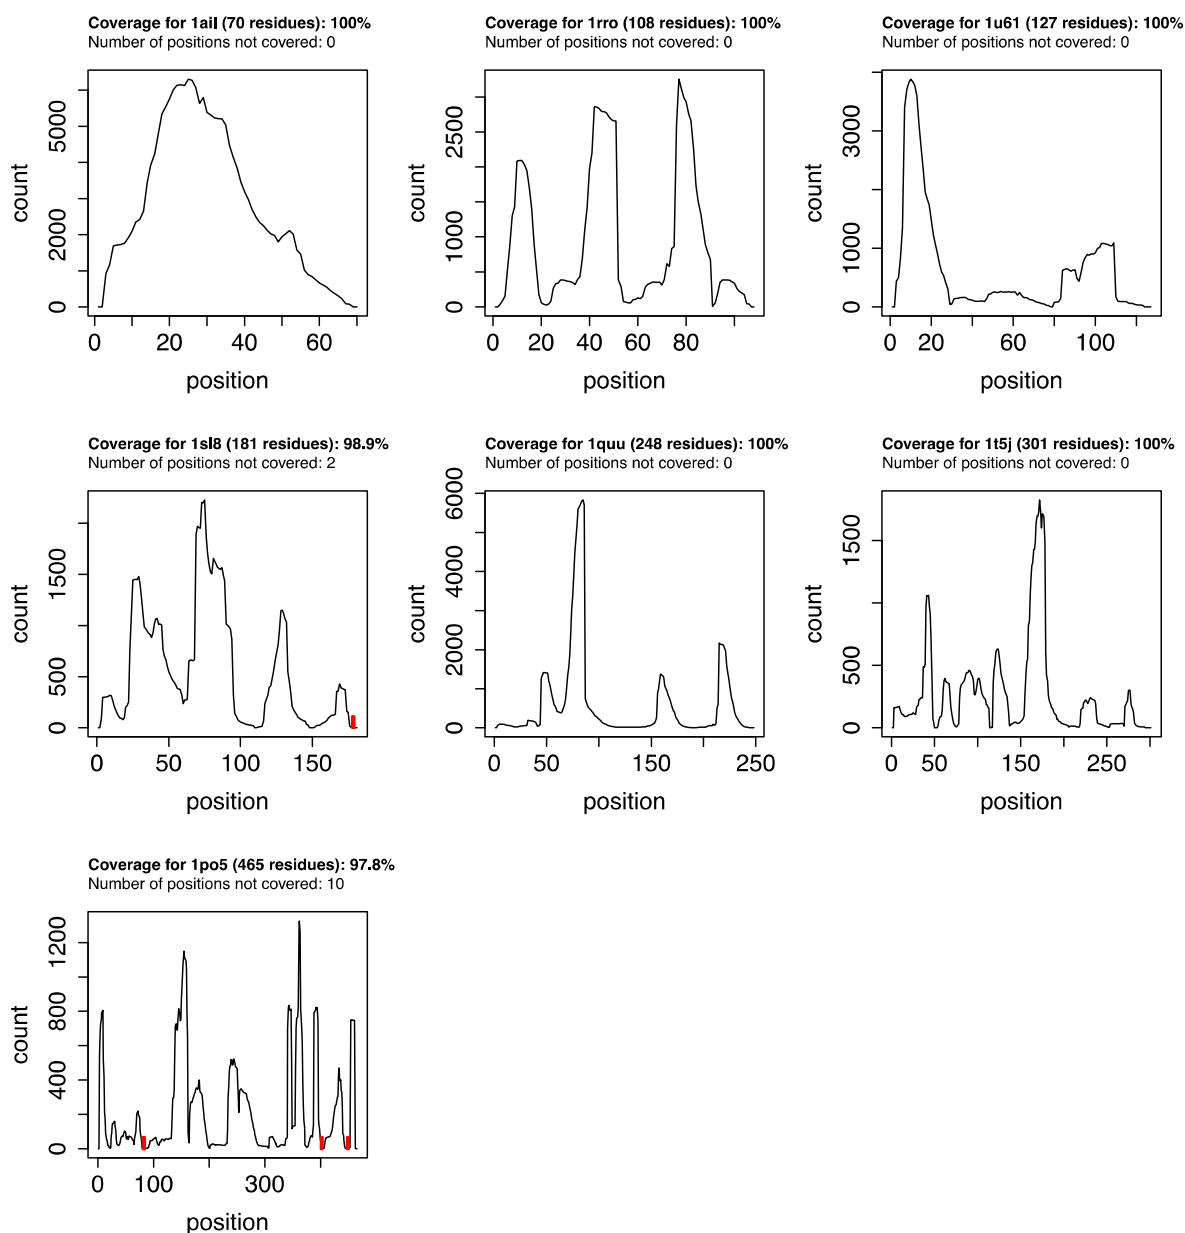

## Supplementary Figure 1.1b

### Protein Block Assignment (PBA) – SCOP Class – all $\beta$

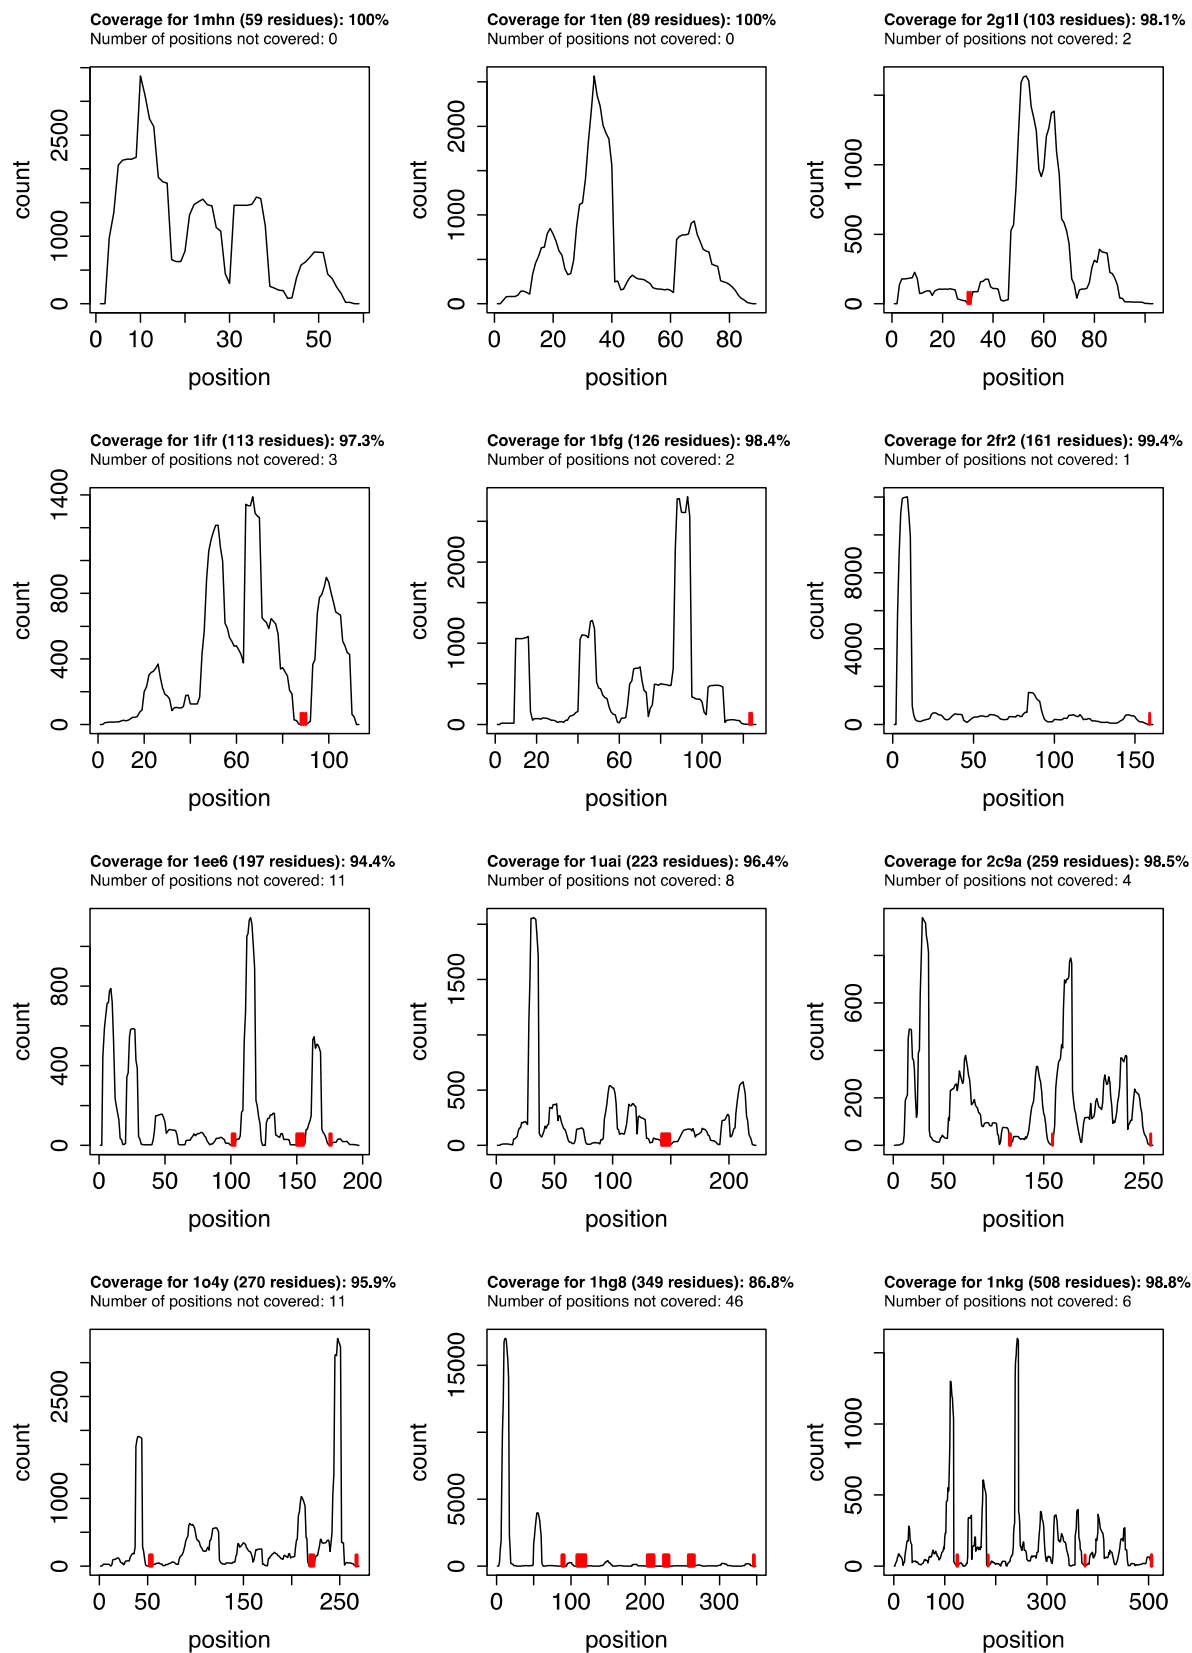

# Supplementary Figure 1.1c

## Protein Block Assignment (PBA) – SCOP Class – $\alpha+\beta$

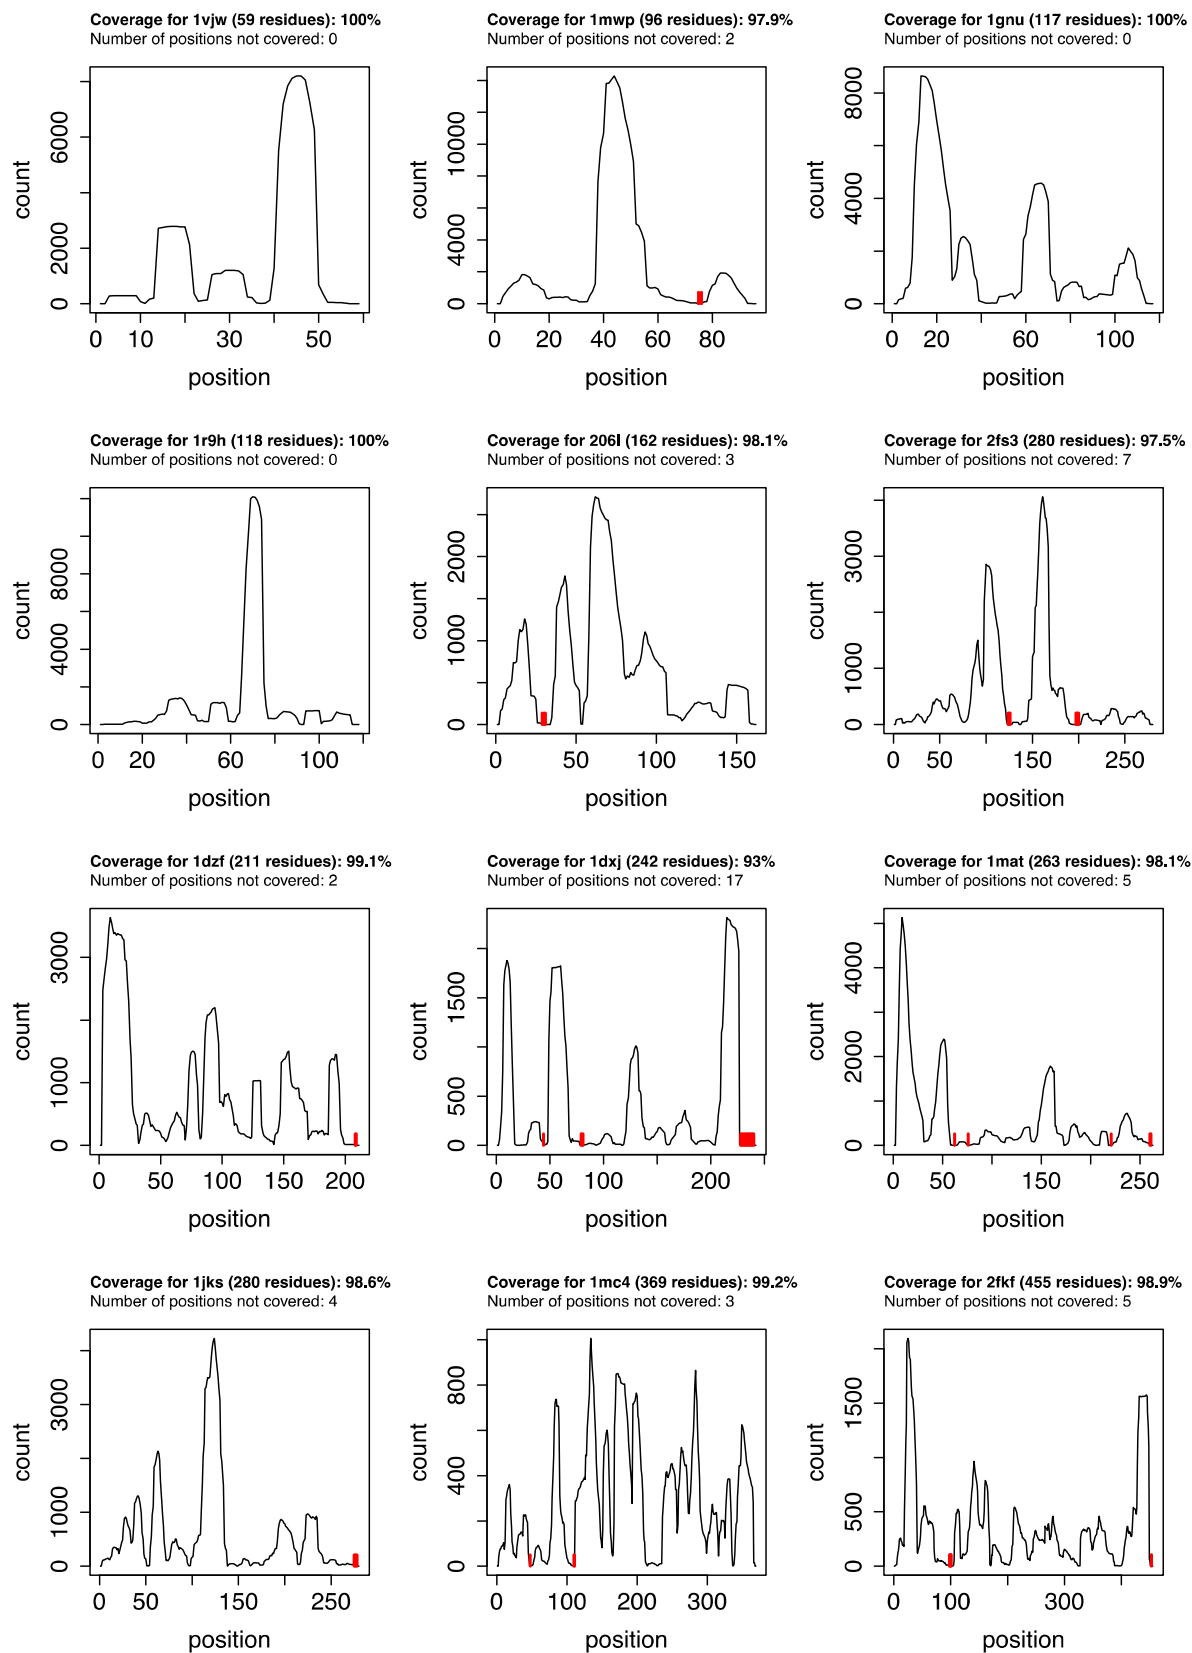

# Supplementary Figure 1.1d

## Protein Block Assignment (PBA) – SCOP Class – $\alpha/\beta$

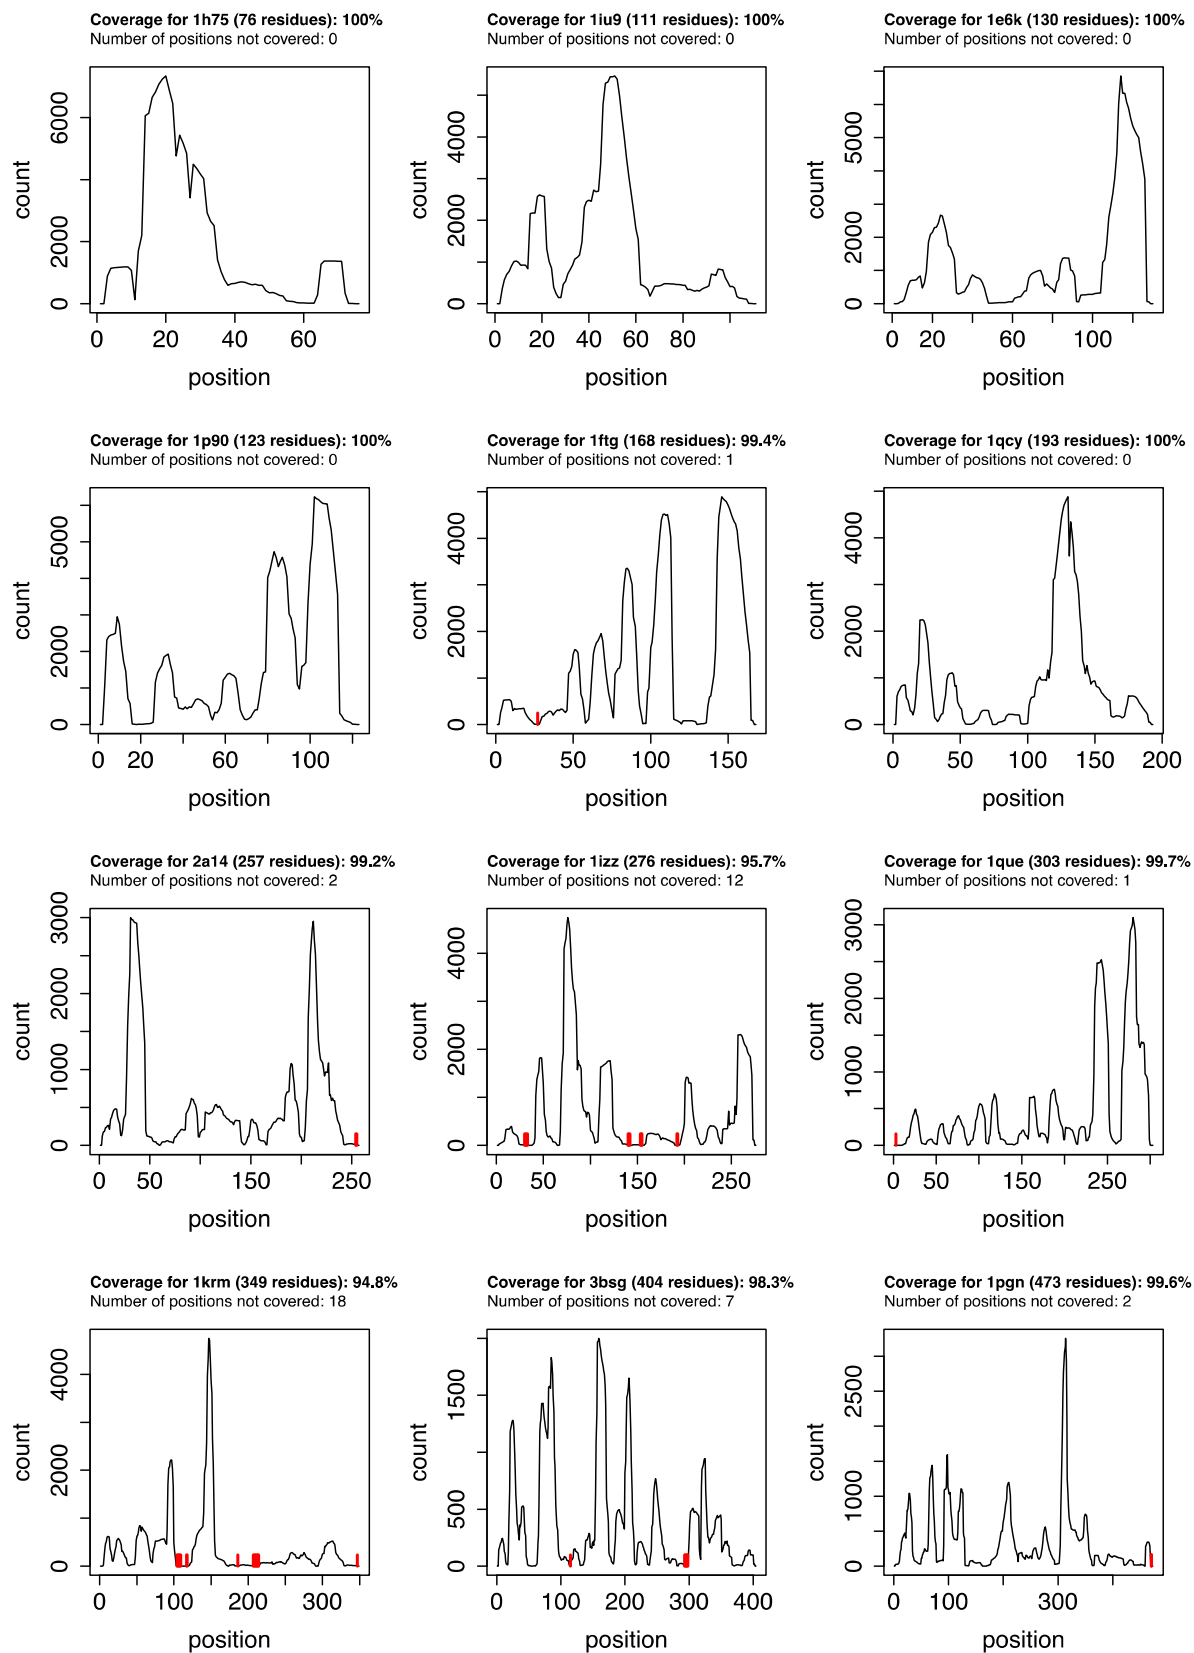

## Supplementary Figure 1.2a

### Protein Block Prediction (PBP) - SCOP Class – all $\alpha$

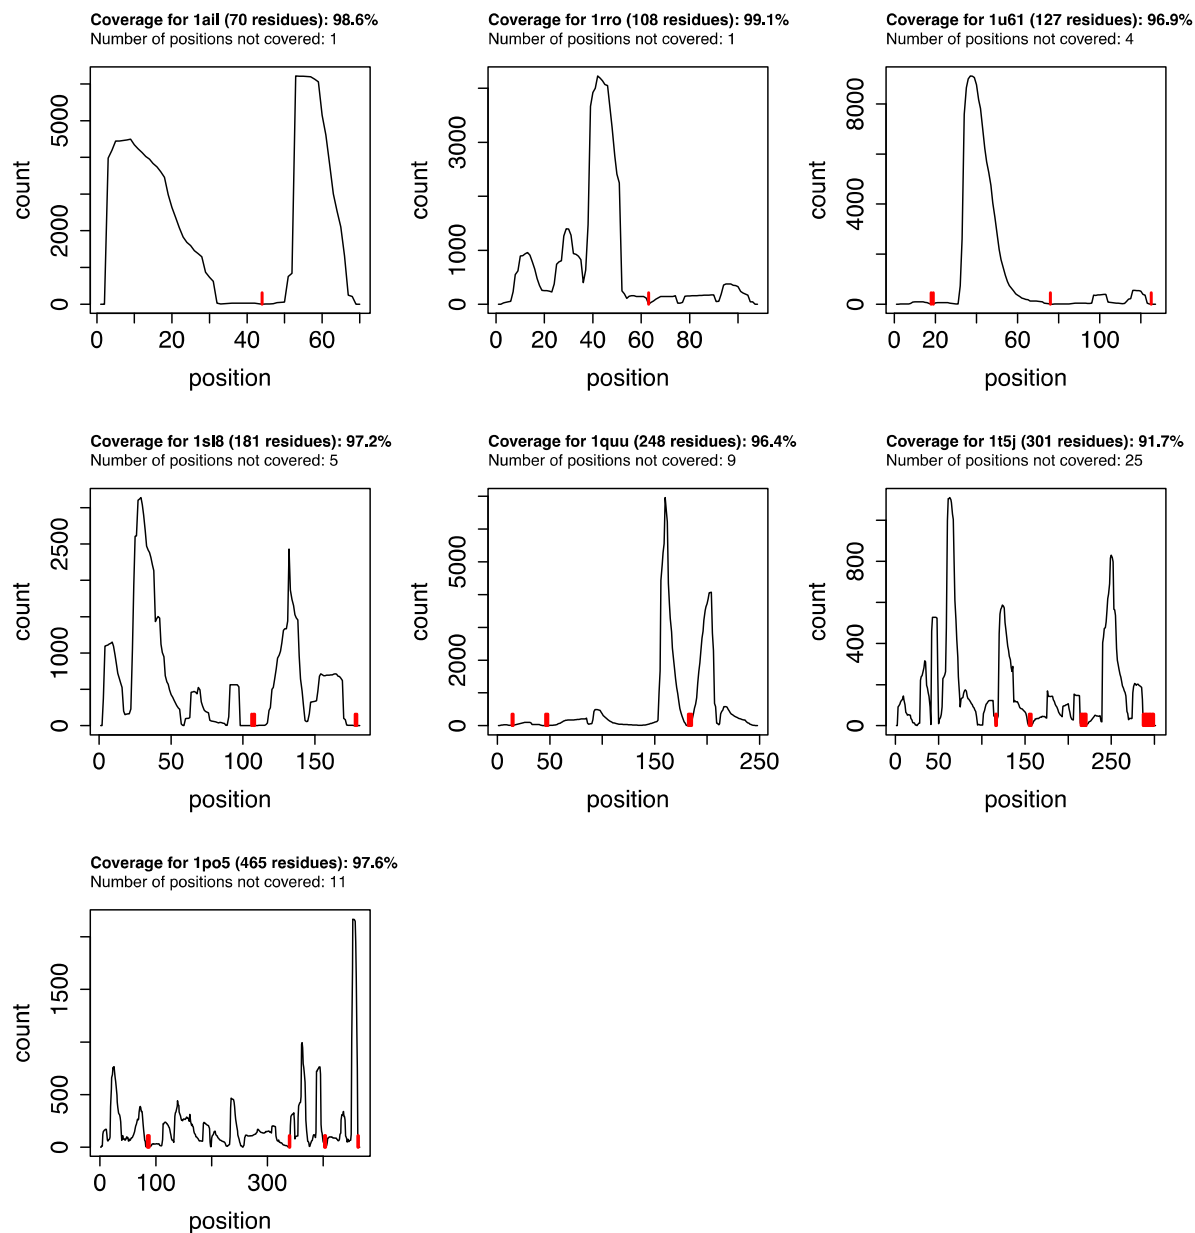

## Supplementary Figure 1.2b

### Protein Block Prediction (PBP) - SCOP Class – all $\beta$

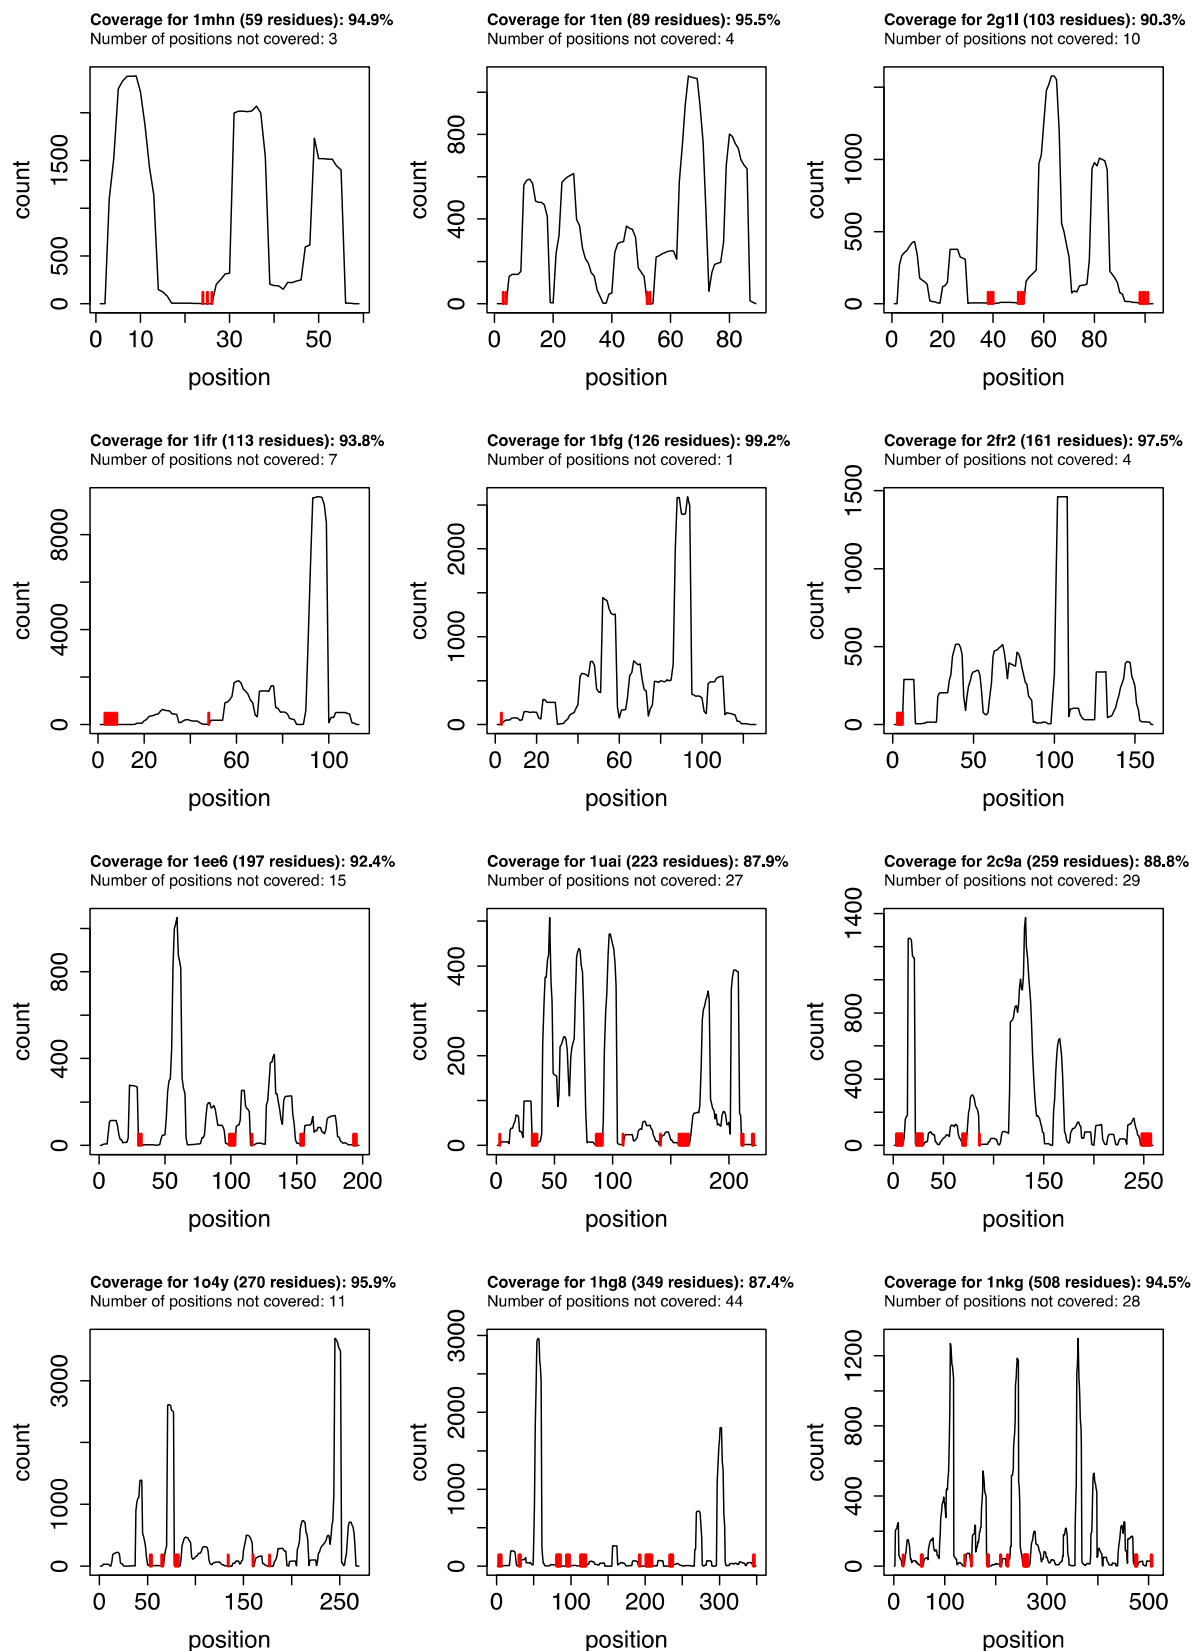

## Supplementary Figure 1.2c

### Protein Block Prediction (PBP) - SCOP Class – $\alpha+\beta$

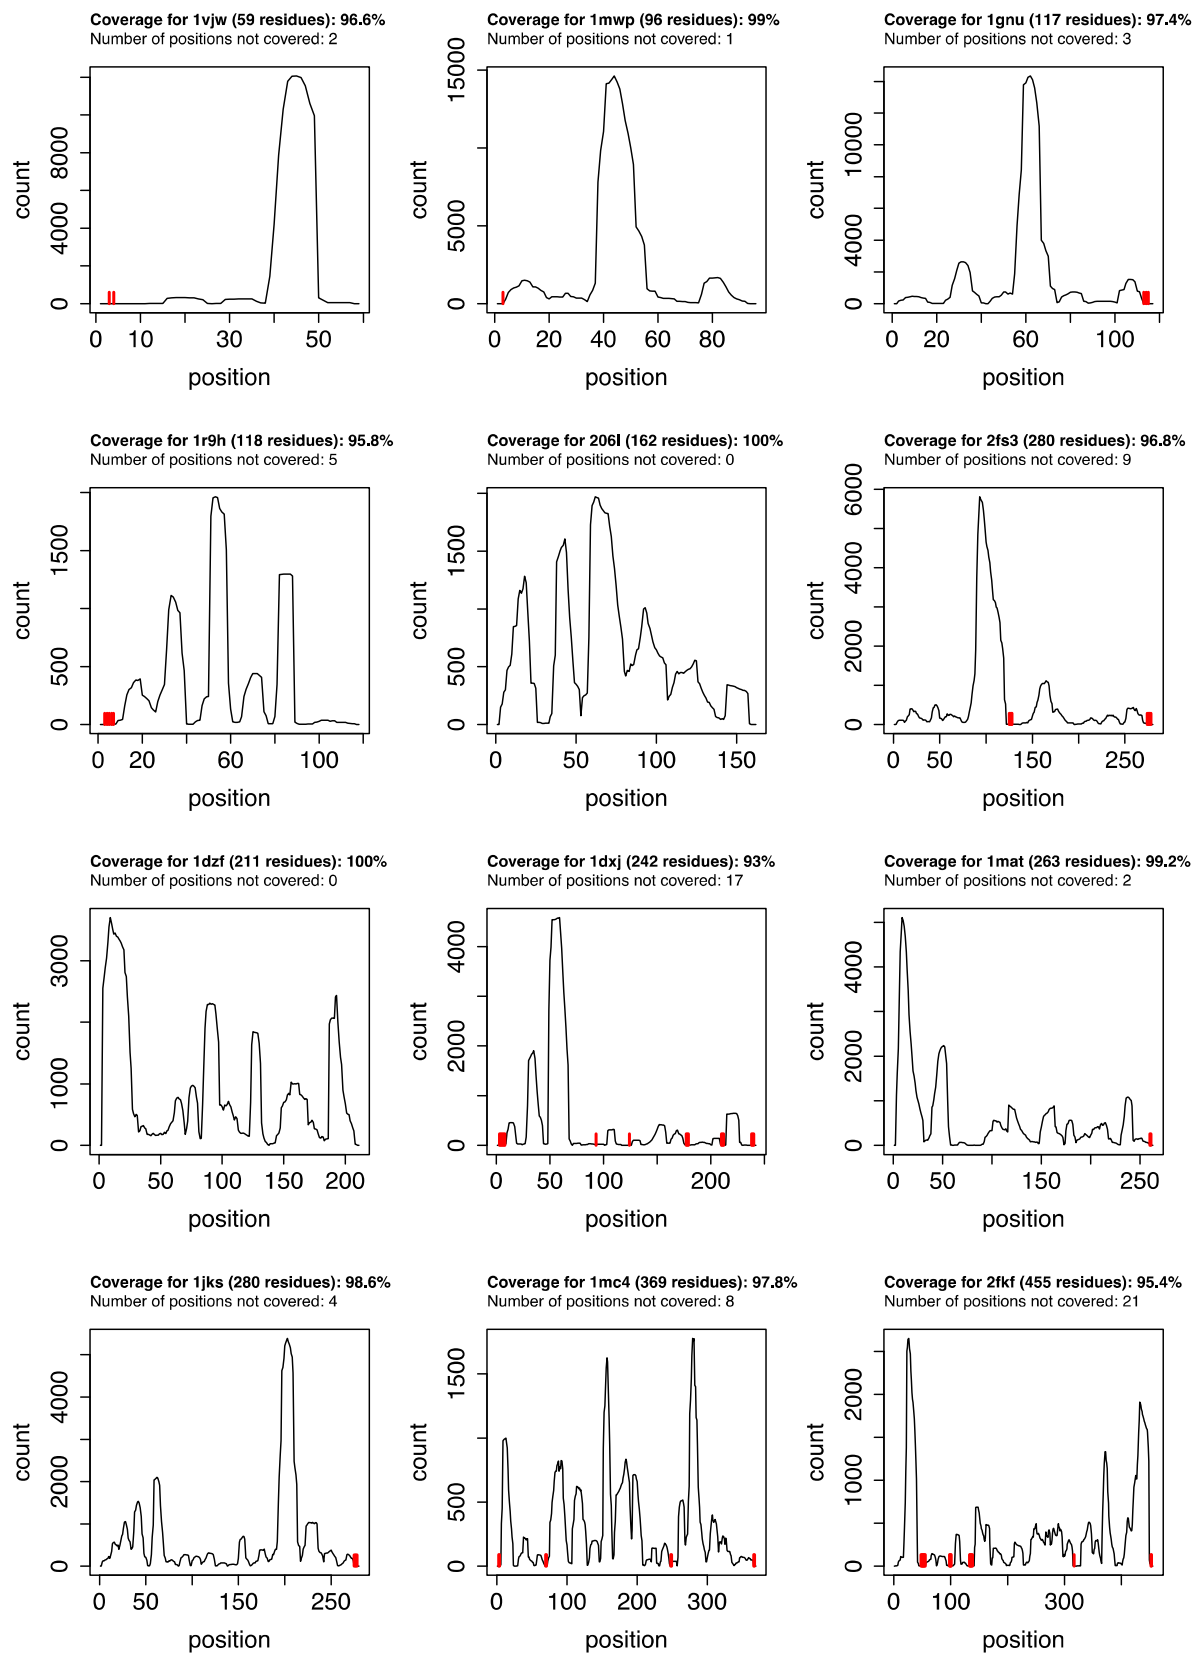

## Supplementary Figure 1.2d

### Protein Block Prediction (PBP) - SCOP Class – $\alpha/\beta$

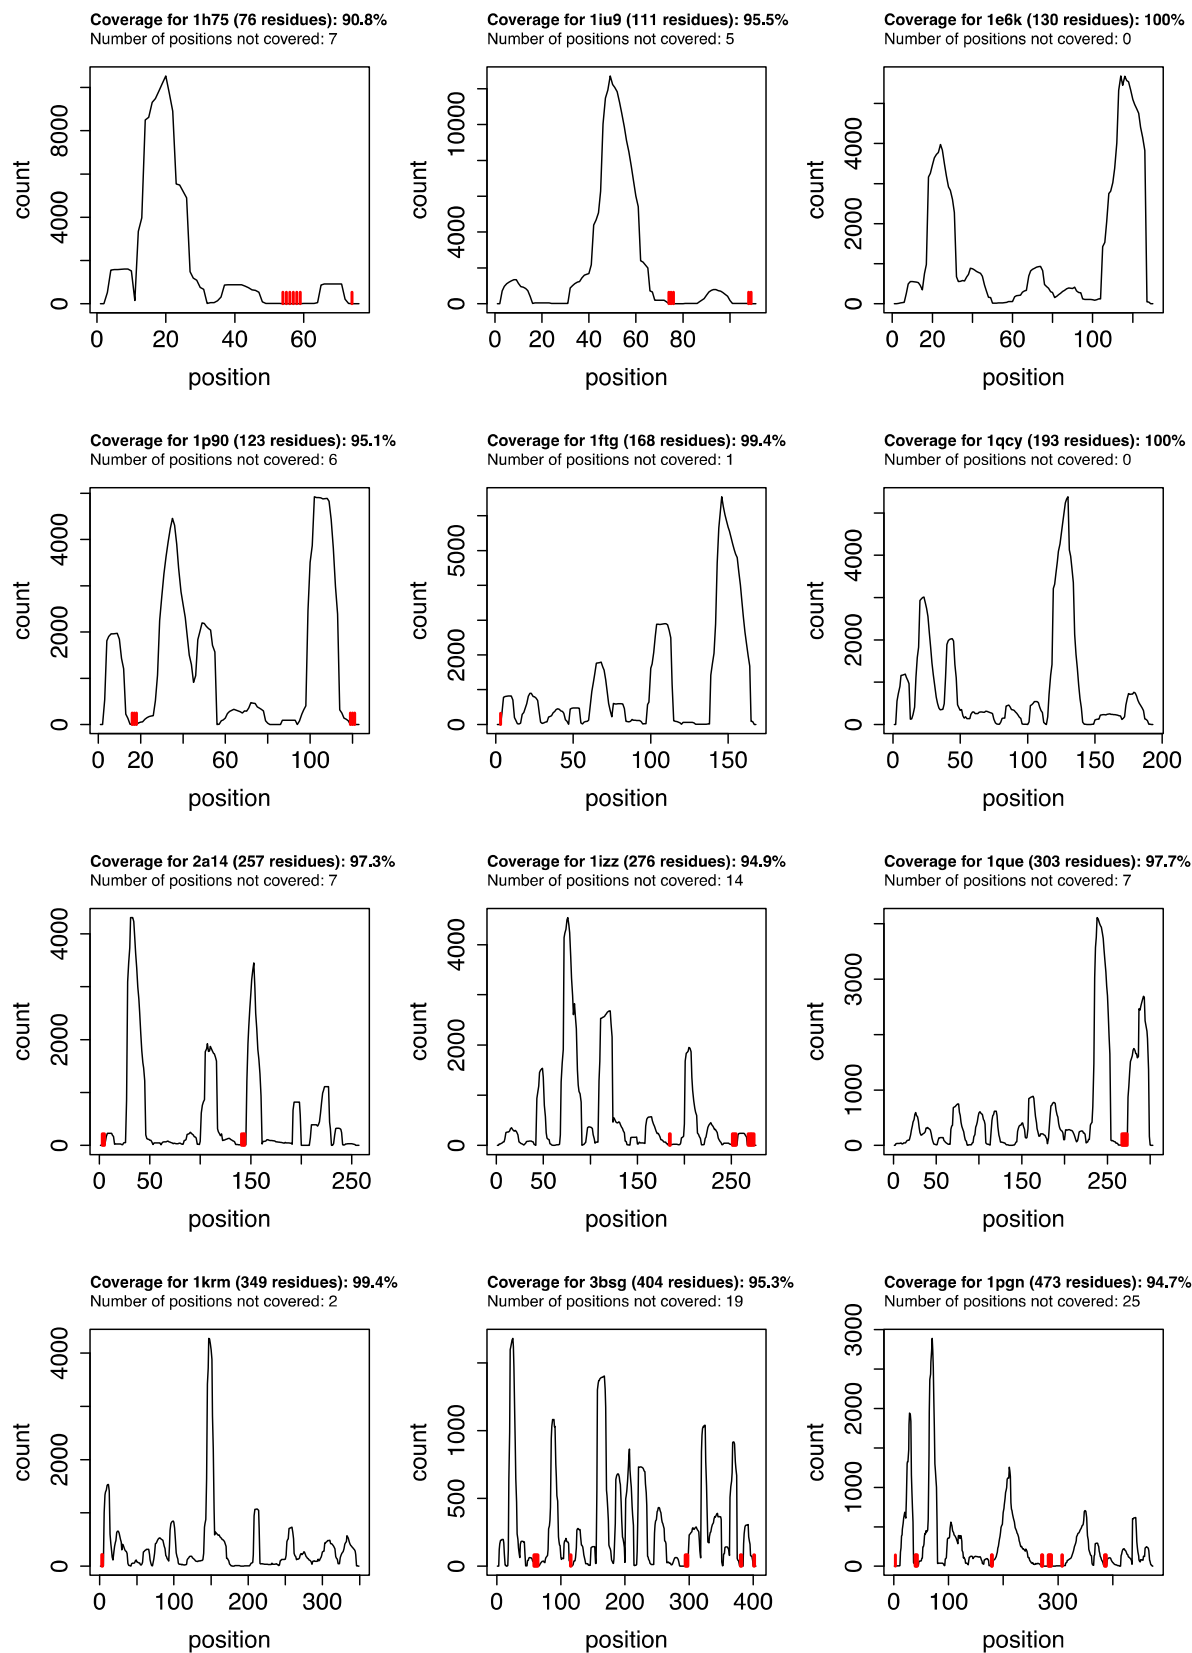

Supplement: Supplementary file 1 [file Supplementary_figure1.pdf]
