# Supplementary material for: Using protein blocks to build custom fragment libraries from protein structures
Source: arXiv:2005.01696 source file (2025-07-19)

## Supplementary Figures 2. Sensitivity and specificity Plots.

The plots under this heading show the co-relation between *rmsd* (2 Å) and three chosen criteria for prioritizing fragment selection, i.e., protein sequence identity, protein sequence similarity and secondary structure identity. The analysis has been performed for both treatment of the query proteins: (1) Protein Block Assignment (PBA) and (2) Protein Block Prediction (PBP). The graphs are further classified into section : (a) SCOP Class –all  $\alpha$ , (b) SCOP Class – all  $\beta$ , (c) SCOP Class -  $\alpha+\beta$  and (d) SCOP Class -  $\alpha/\beta$ .

### Supplementary Figure 2.1a

Protein Block Assignment (PBA) - SCOP Class – all  $\alpha$

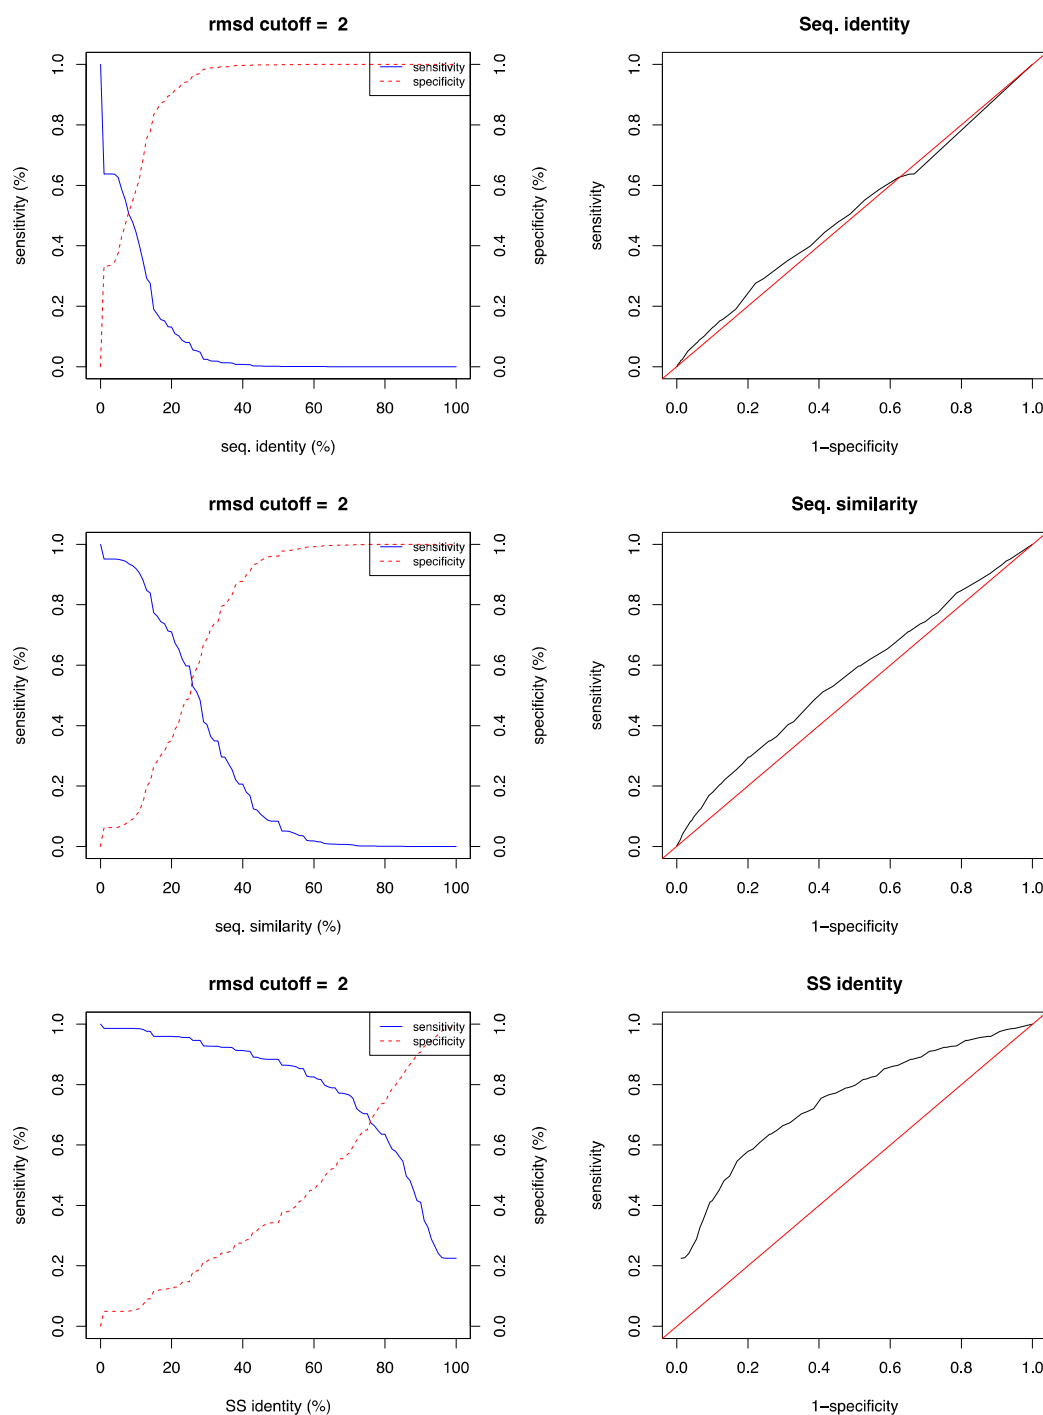

## Supplementary Figure 2.1b

Protein Block Assignment (PBA) – SCOP Class – all  $\beta$

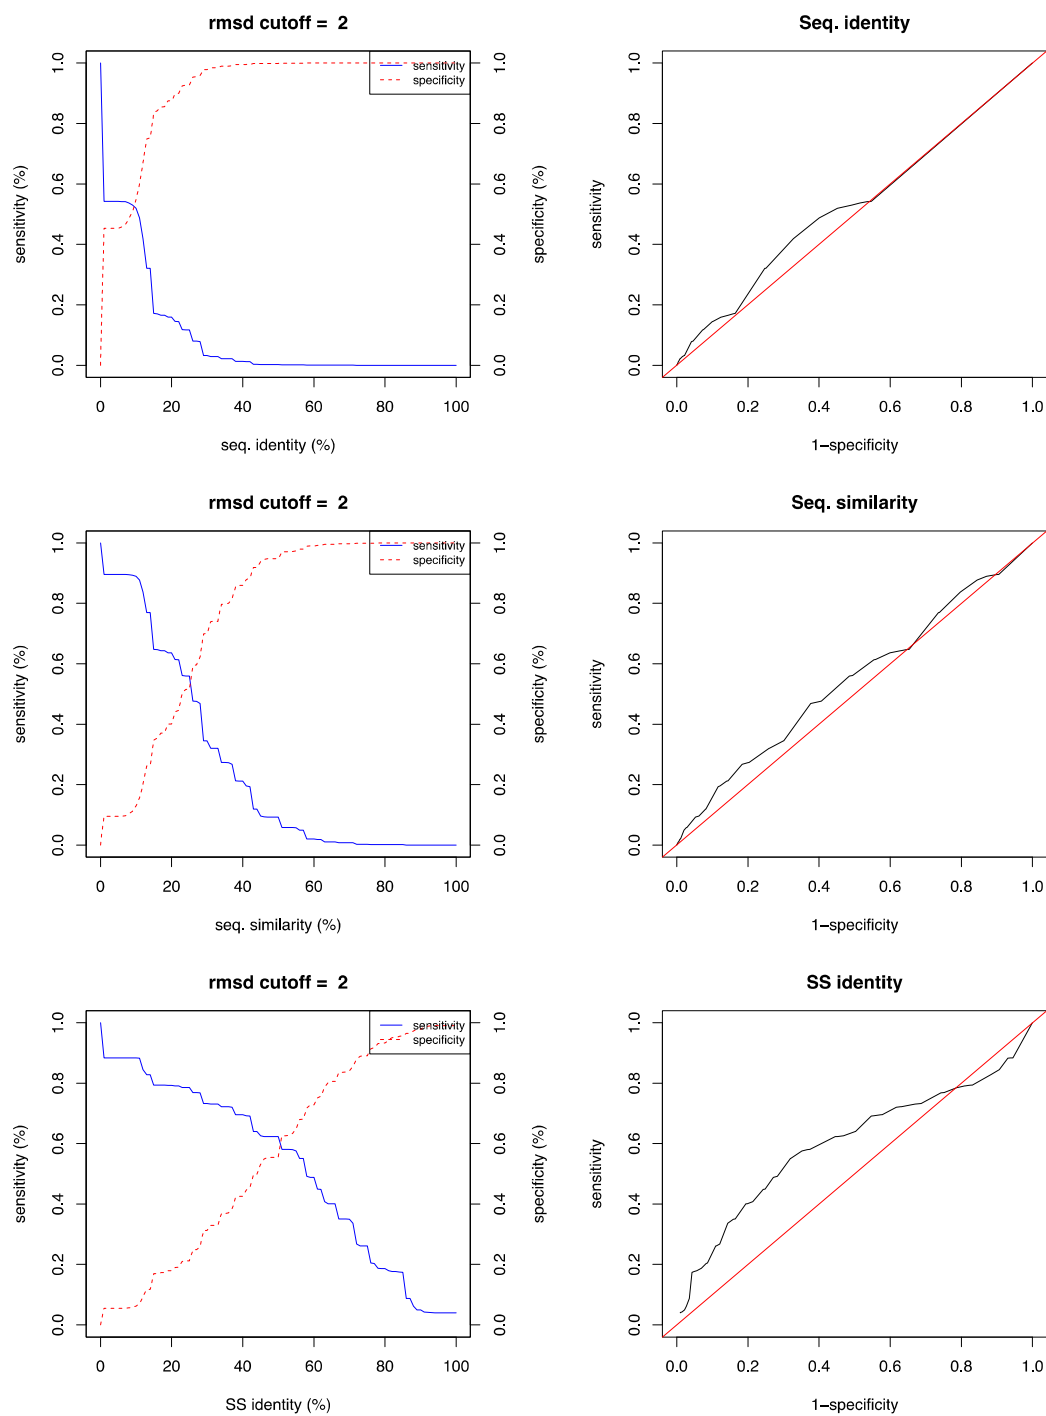

## Supplementary Figure 2.1c

Protein Block Assignment (PBA) – SCOP Class –  $\alpha+\beta$

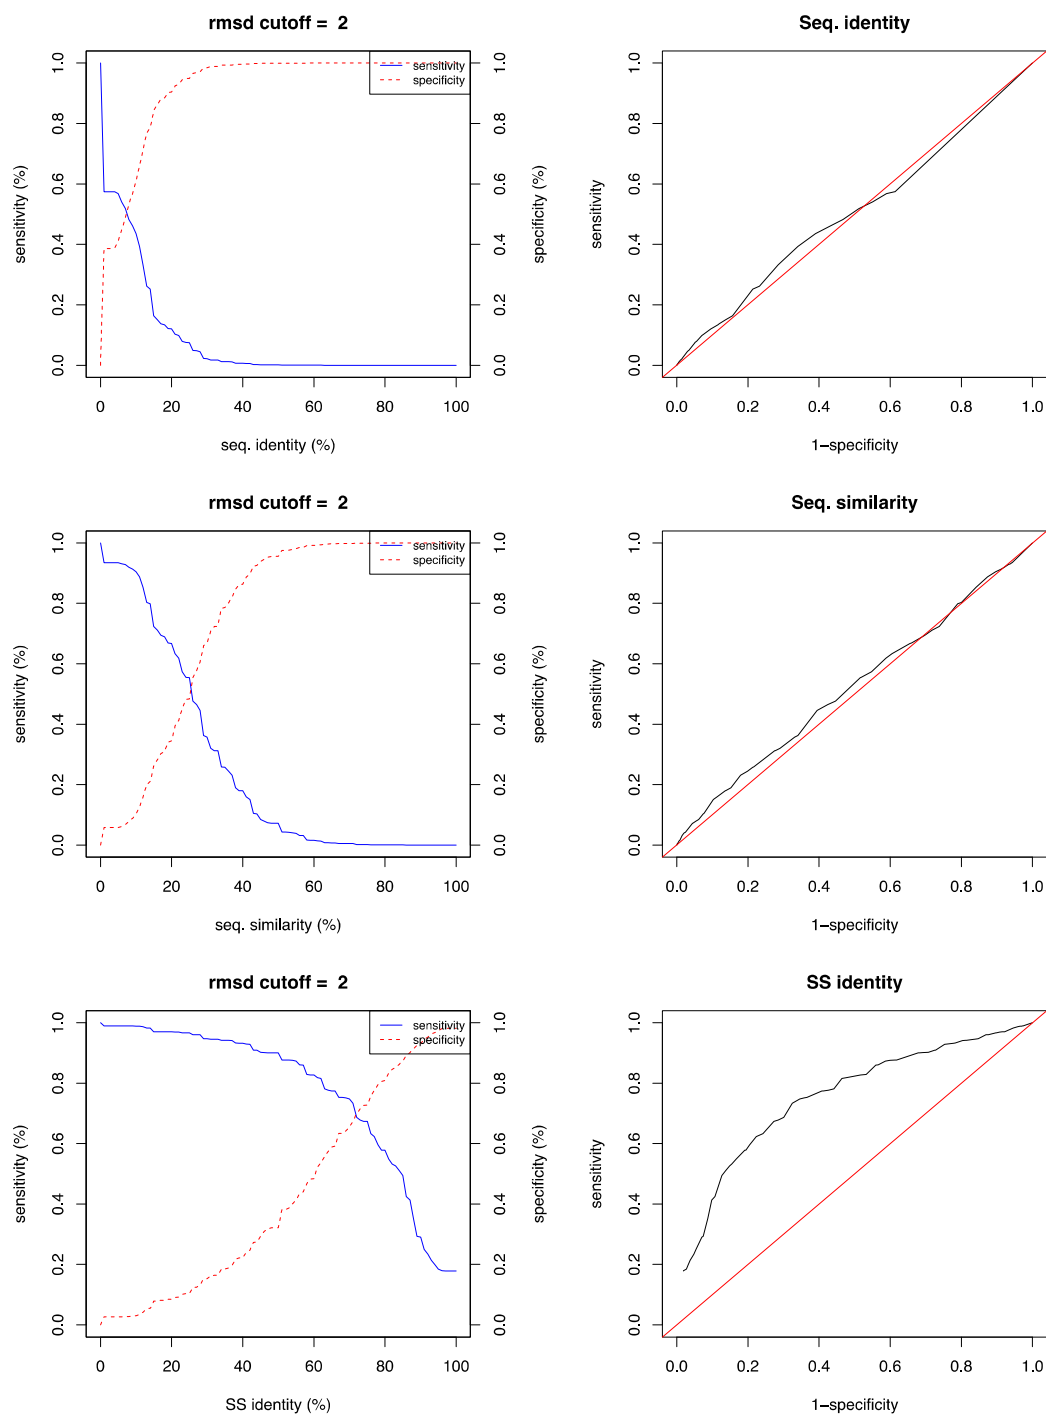

## Supplementary Figure 2.1d

Protein Block Assignment (PBA) – SCOP Class –  $\alpha/\beta$

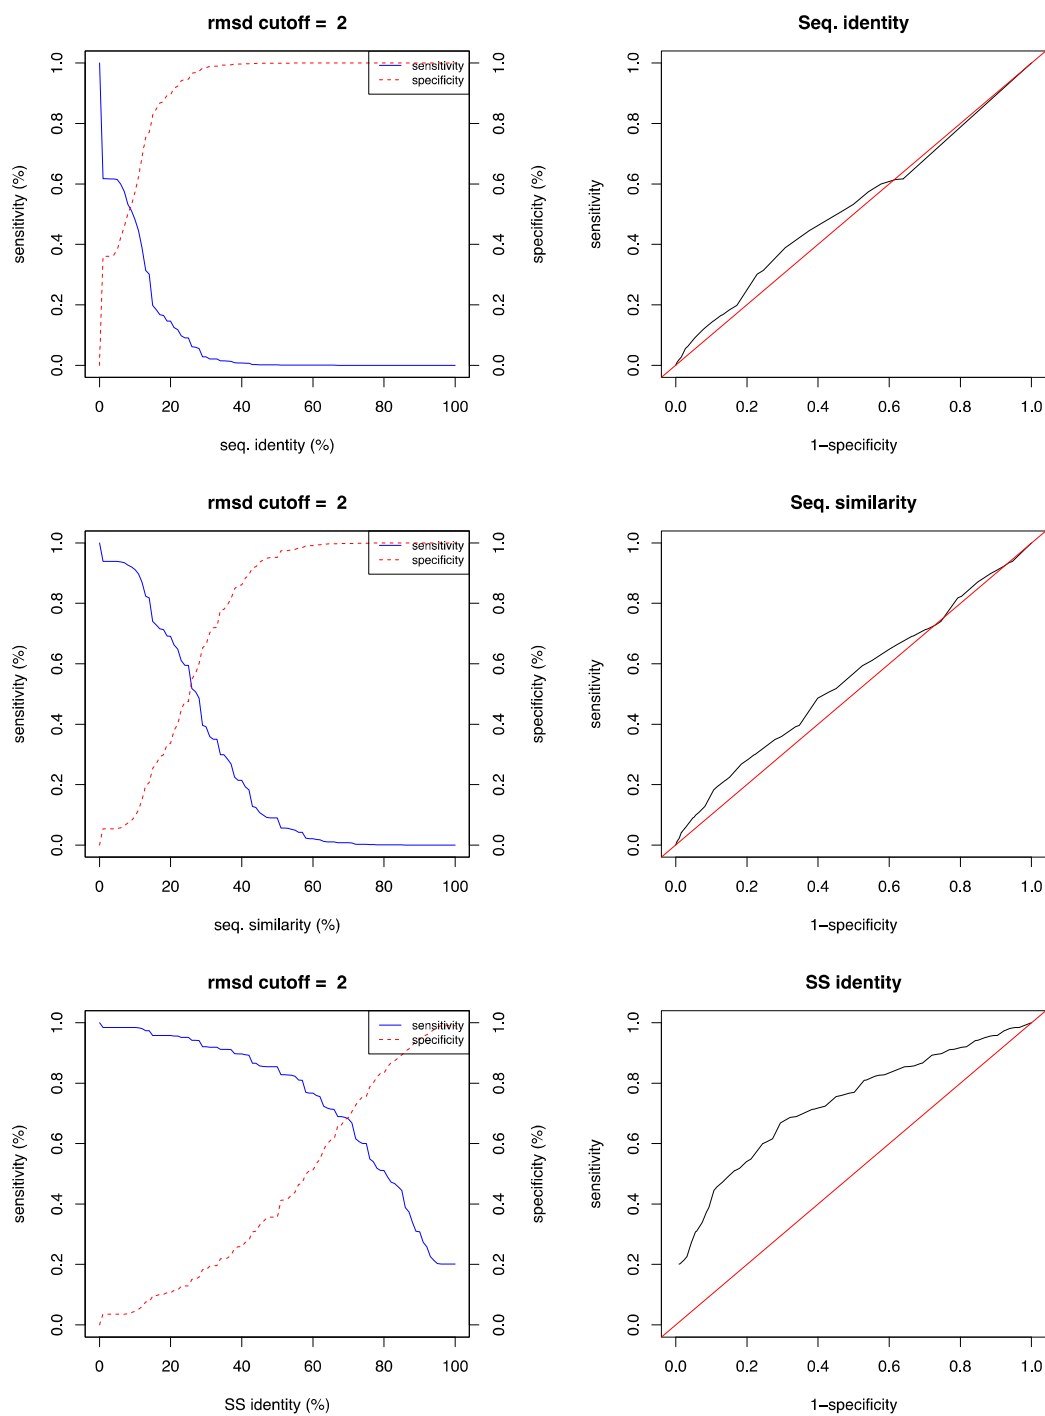

## Supplementary Figure 2.2a

Protein Block Prediction (PBP) - SCOP Class – all  $\alpha$

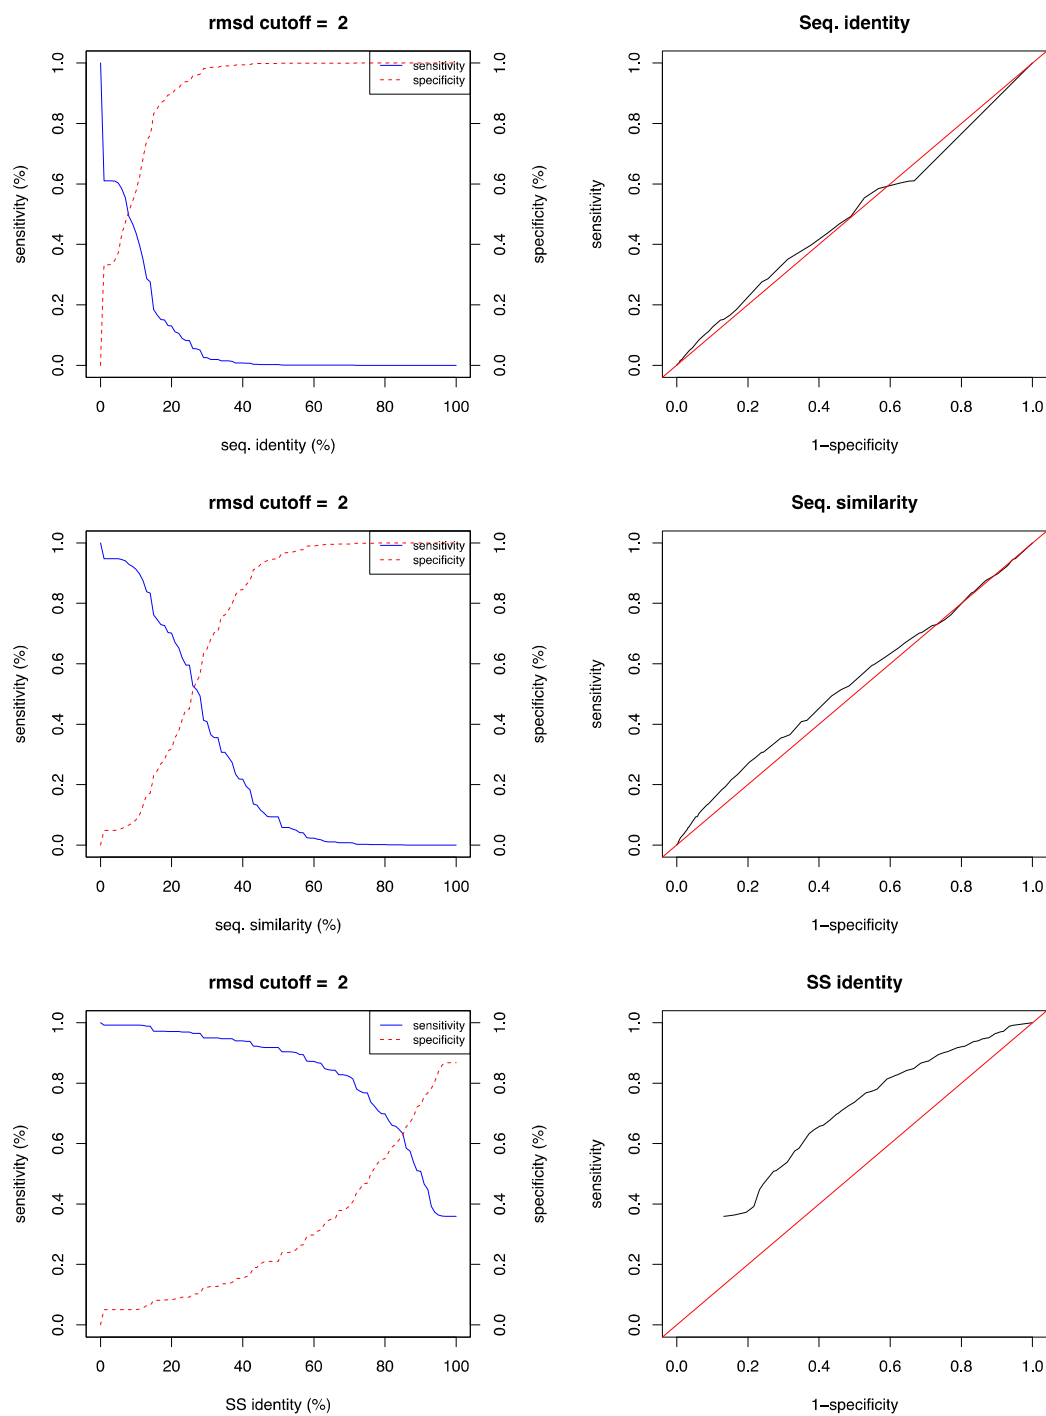

## Supplementary Figure 2.2b

Protein Block Prediction (PBP) - SCOP Class – all  $\beta$

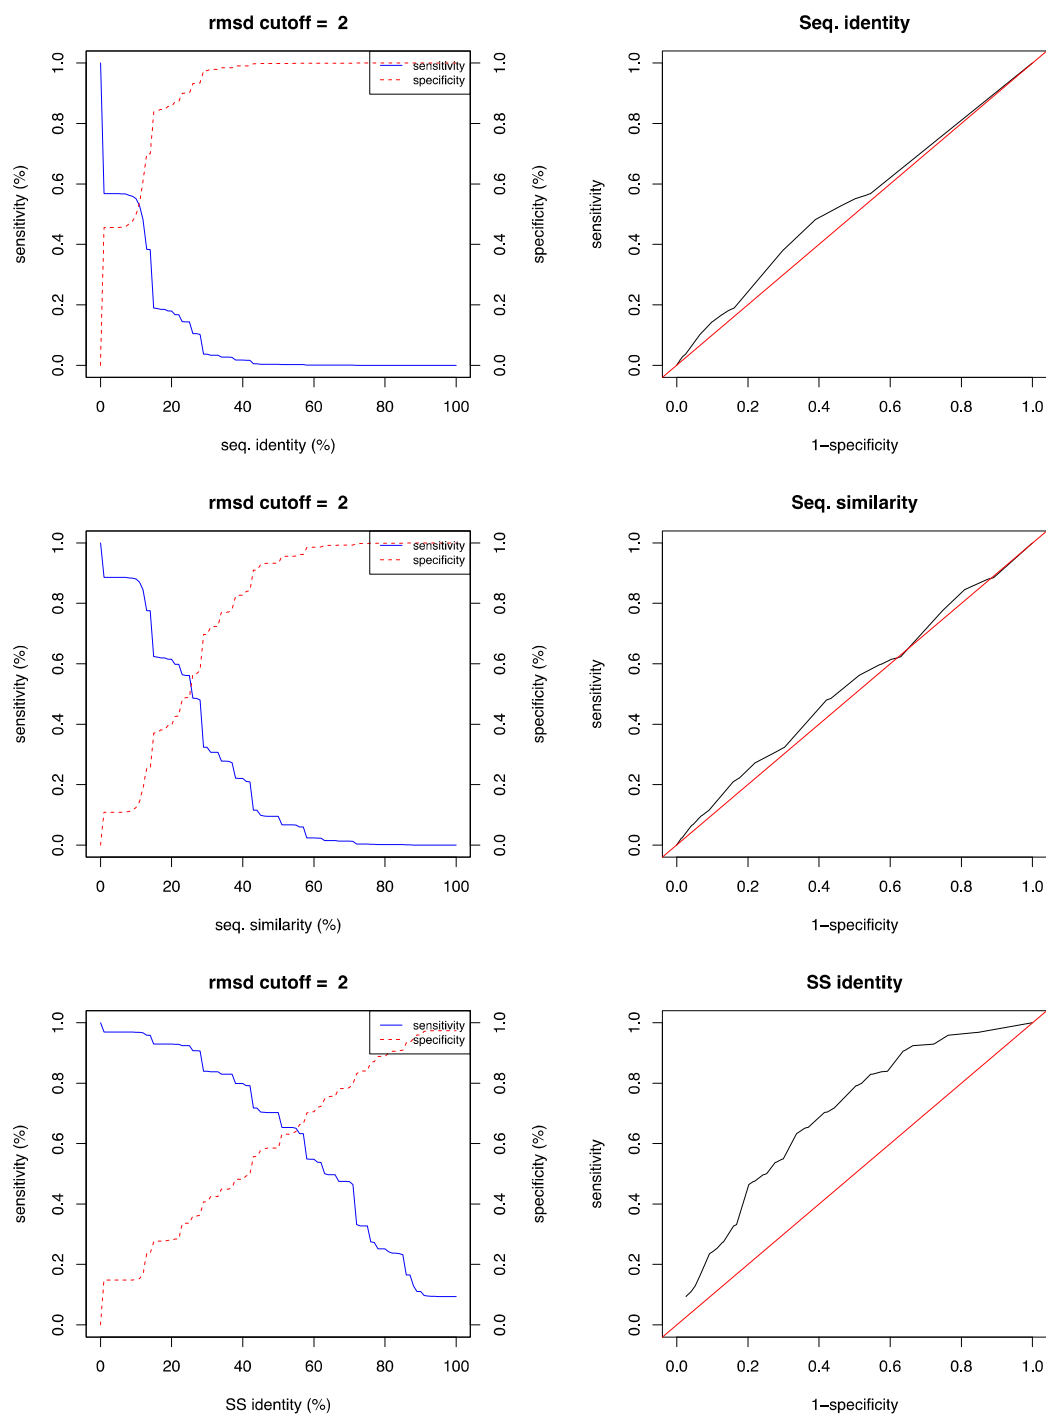

## Supplementary Figure 2.2c

Protein Block Prediction (PBP) - SCOP Class –  $\alpha+\beta$

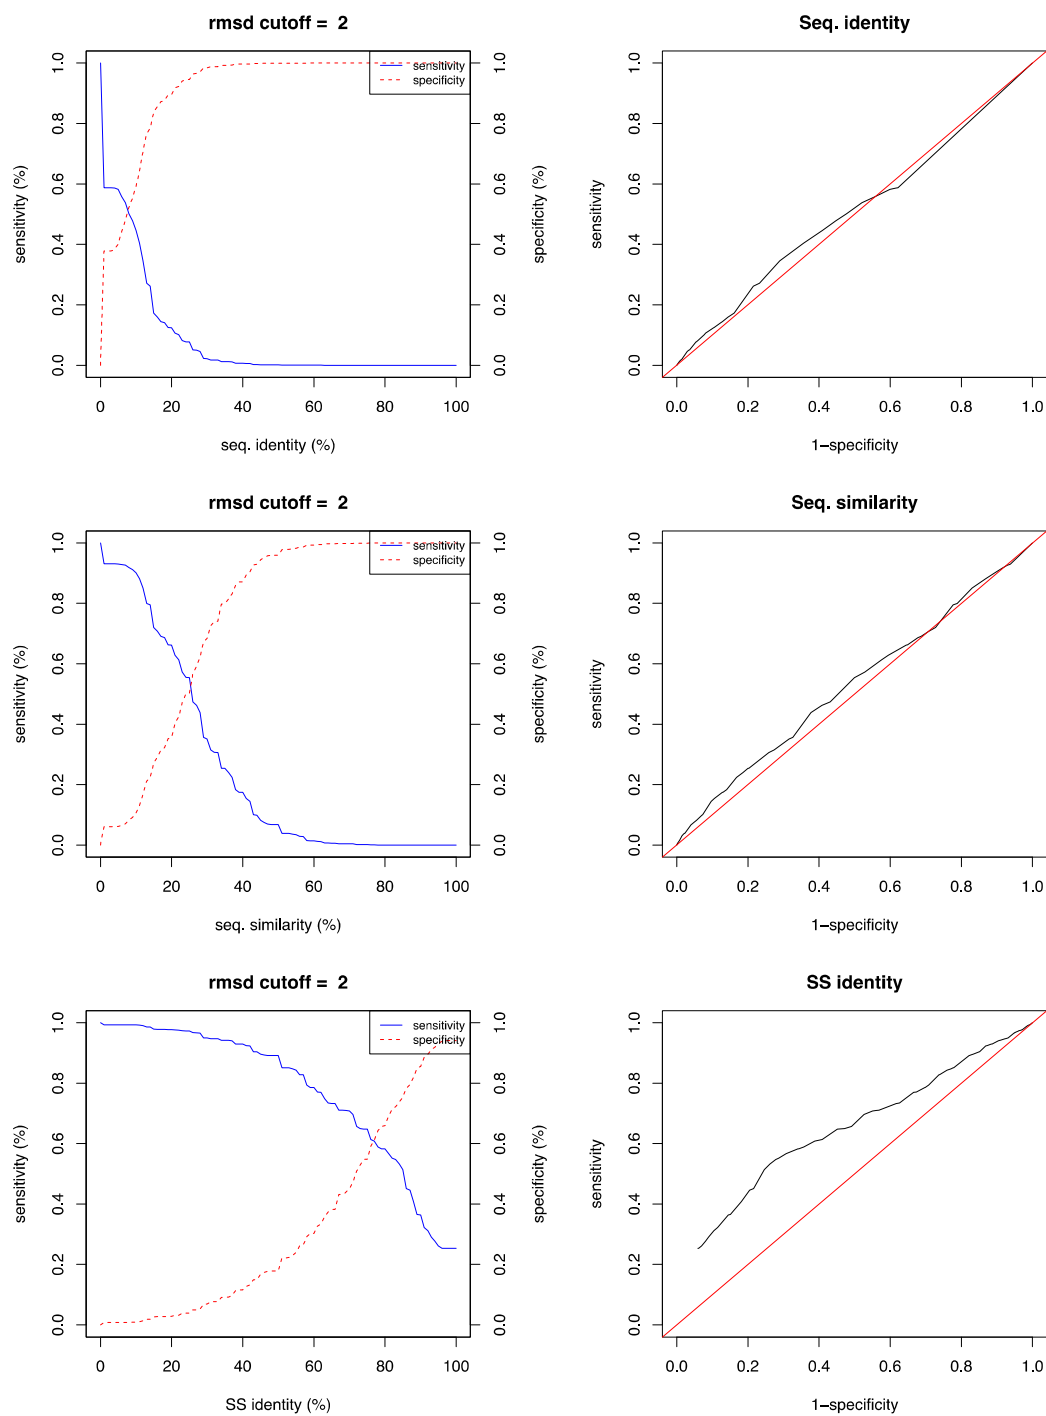

## Supplementary Figure 2.2d

Protein Block Prediction (PBP) - SCOP Class –  $\alpha/\beta$

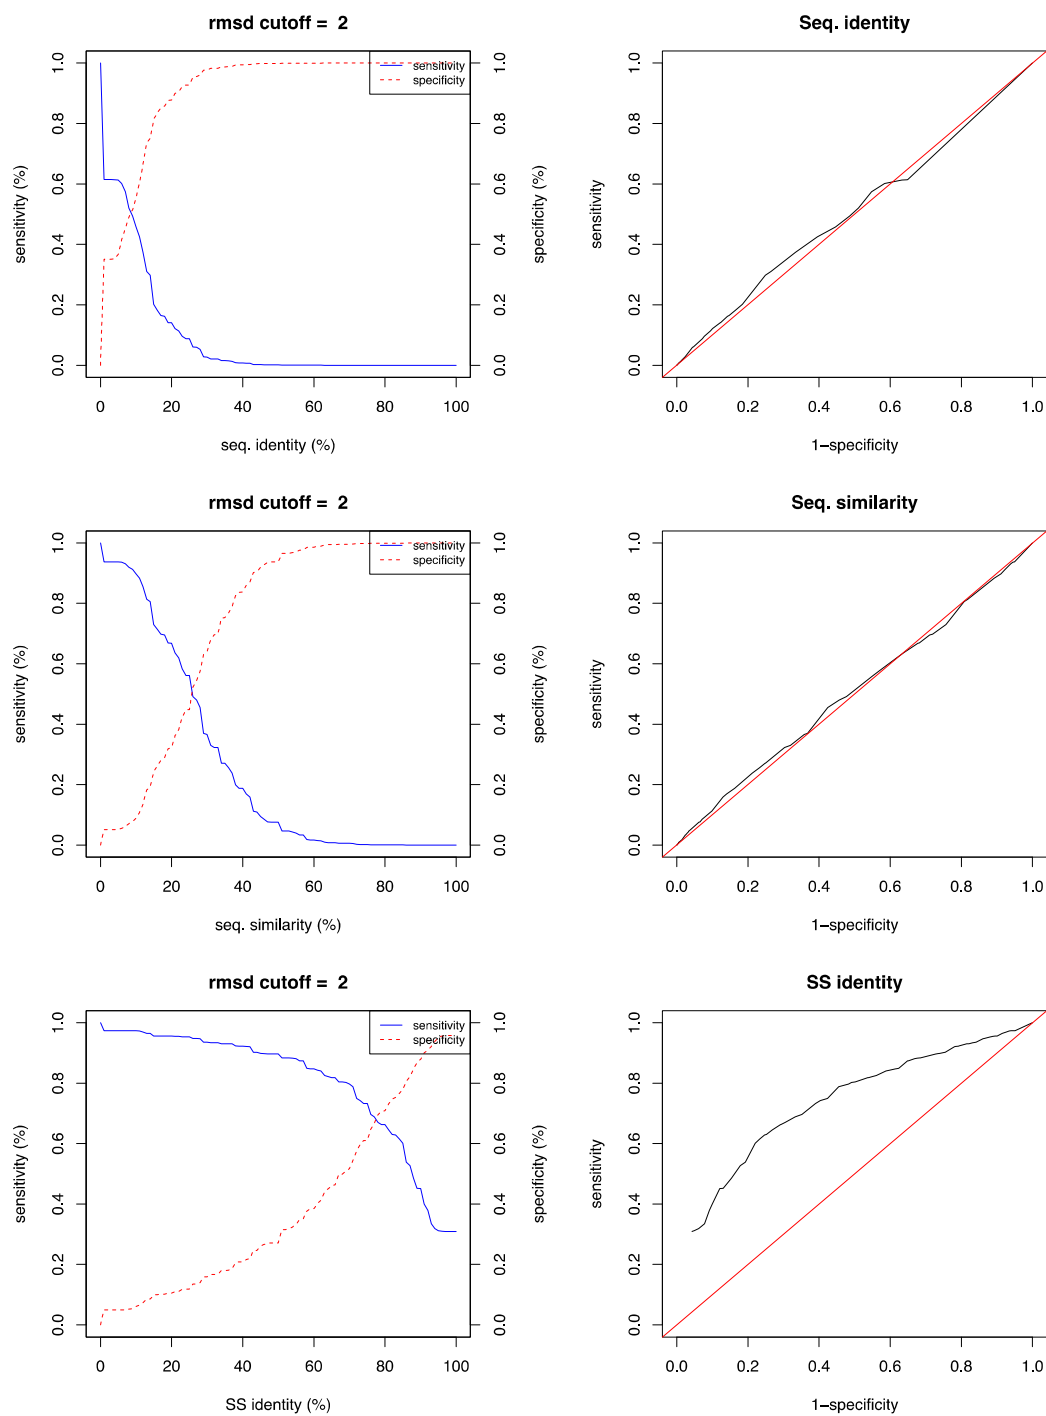

Supplement: Supplementary file 2 [file Supplementary_figure2.pdf]
